# Supplementary material for: Gate field effects on the topological insulator BiSbTeSe2 interface
Source: arXiv:1910.06994 ancillary file (2020-06-08)
Supplement: Supplementary file 1 [file supplemental_info.pdf]

# Gate field effects on the topological insulator $\mathrm{BiSbTeSe_2}$ interface

Shuanglong Liu,[1,2] Yang Xu,[3,a)] Yun-Peng Wang,[1,2,b)] Yong P. Chen,[3,4,5,6] James N. Fry,[1] and Hai-Ping Cheng[1,2,7,c)]

[1)] *Department of Physics, University of Florida, Gainesville, Florida 32611, USA*

[2)] *Quantum Theory Project, University of Florida, Gainesville, Florida 32611, USA*

[3)] *Department of Physics and Astronomy, Purdue University, West Lafayette, Indiana, 47907, USA*

[4)] *School of Electrical and Computer Engineering, Purdue University, West Lafayette, Indiana, 47907, USA*

[5)] *Birck Nanotechnology Center, Purdue University, West Lafayette, Indiana, 47907, USA*

[6)] *Purdue Quantum Science and Engineering Institute, Purdue University, West Lafayette, Indiana, 47907, USA*

[7)] *Center for Molecular Magnetic Quantum Materials, University of Florida, Gainesville, Florida 32611, USA*

(Dated: 27 December 2019)

Interfaces between two topological insulators are of fundamental interest in condensed matter physics. Inspired by experimental efforts, we study interfacial processes between two slabs of $BiSbTeSe_2$ (BSTS) via first principles calculations. Topological surface states are absent for the BSTS interface at its equilibrium separation, but our calculations show that they appear if the inter-slab distance is greater than 6 Å. More importantly, we find that topological interface states can be preserved by inserting two or more layers of hexagonal boron nitride between the two BSTS slabs. In experiments, the electric current tunneling through the interface is insensitive to back gate voltage when the bias voltage is small. Using a first-principles based method that allows us to simulate a back gate, we show that at low bias the extra charge induced by a gate voltage resides on the surface that is closest to the gate electrode, leaving the interface almost undoped. This provides clues to understand the origin of the observed insensitivity of transport properties to back voltage at low bias. Our study resolves a few questions raised in experiment, which does not yet offer a clear correlation between microscopic physics and transport data. We provide a road map for the design of vertical tunneling junctions involving the interface between two topological insulators.

[a]Current address: Applied and Engineering Physics, Cornell University, Ithaca, New York 14853, USA

[b]Current address: School of Physical Science and Electronics, Central South University, Changsha, Hunan, 410012, China

[c]Electronic mail: hping@ufl.edu

Using the dry transfer method, we stacked two flakes of BSTS to form a vertical tunneling junction on a highly $p$-doped Si substrate coated with 300 nm $SiO_2$. The $p$-doped Si substrate permits a back gate electric field. The lower BSTS slab is about 15 nm thick and the upper one is thicker than 30 nm. The lower BSTS slab is grounded and a bias voltage is applied between the two BSTS slabs. A schematic of the BSTS vertical tunneling junction is shown the upper inset of Fig. S1. The main figure shows the electric current $I$ through the interface versus the bias voltage $V_{\text{tb}}$ for the system under different back gate voltages $V_{\text{bg}}$. Differential conductance versus gate voltage for the system at zero bias voltage is plotted in the lower inset. These results clearly show that the electron transport properties are not sensitive to the back gate voltage $V_{\text{bg}}$ when the bias voltage is small, as explained in the main text. The gate field dependence of electric current becomes stronger at higher bias voltages. One possible explanation to such a dependence is also given towards the end of the main text but it is not well understood. Further finite bias calculations are needed to take non-equilibrium effects into account.

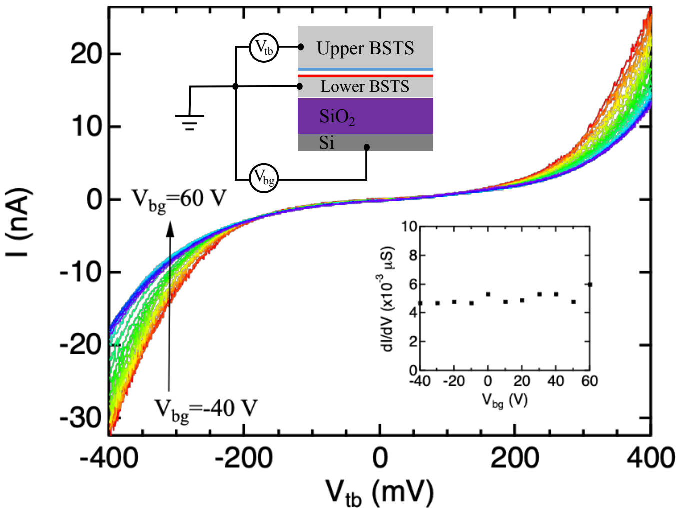


FIG. S1. Electric current versus bias voltage for the BSTS vertical tunneling junction under different gate voltages. Different color represents different gate voltage. Inset one: schematic experimental setup for electron transport measurement. The interface between the two slabs is highlighted by the thick lines. The thick blue (red) line is from the upper (lower) BSTS slab. Inset two: differential conductance ($\mathrm{d}I/\mathrm{d}V$) versus gate voltage for the junction under zero bias.

Fig. S2 shows the atomic configuration and the band structure of the special random BSTS bulk. The lattice constants are $a = 8.395$ Å, $b = 4.188$ Å, $c = 29.390$ Å, $\alpha = 90.00°$, $\beta = 90.00°$, and $\gamma = 120.00°$. It has an indirect band gap of $E_g \approx 0.18$ eV for which the

spin-orbit interaction is included.

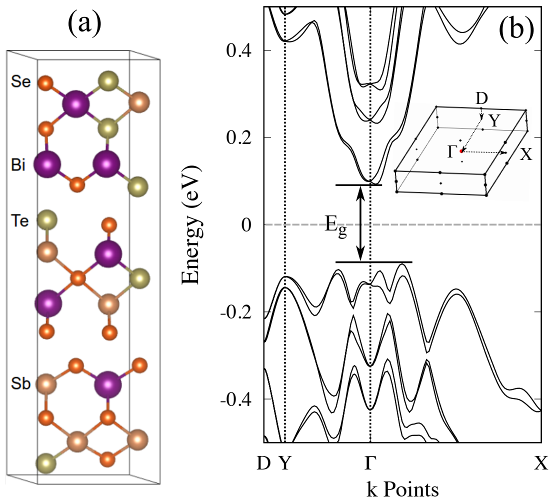


FIG. S2. (a) The unit cell and (b) the band structure of the special random BSTS bulk. The solid black lines in panel (a) are the cell boundaries. In panel (b), the Fermi energy is set to zero and the band gap $E_g$ is indicated by the two headed arrow. The $k$ path in the first Brillouin zone is illustrated in the inset.

For a 3D time reversal topological insulator, the topological invariants $(v; v_1, v_2, v_3)$ can be found by[1]

$$v = \Delta(k_i = 0.0) + \Delta(k_i = 0.5) \text{ mod } 2,\ i = 1, 2, 3, \tag{S1}$$

$$v_i = \Delta(k_i = 0.5). \tag{S2}$$

Each $\Delta(k_i)$ is a $\mathbb{Z}_2$ number defined at the reciprocal plane $k_i$. It can obtained by examining the number of crossings of hybrid Wannier charge centers by a line from $k = 0.0$ to $k = 0.5$. Fig. S3 shows the evolution of hybrid Wannier charge centers of the special random BSTS bulk. Since the number of crossings for $k_x = 0.0$ [$k_x = 0.5$] is odd [even], $\Delta(k_x = 0.0) = 1$ [$\Delta(k_x = 0.5) = 0$]. Similarly, $\Delta(k_y = 0.0) = 1$, $\Delta(k_y = 0.5) = 0$, $\Delta(k_z = 0.0) = 1$, and $\Delta(k_z = 0.5) = 0$. It follows that $(v; v_1, v_2, v_3) = (1; 0, 0, 0)$. As such, our model BSTS represents a strong topological insulator.

Fig. S4(a) shows the band structure of a 6-quinlayer thick BSTS slab without spin-orbit interaction, as calculated by the VASP package. In this case, there is an energy gap of 0.103 eV at the Γ point of the Brillouin zone. When the spin-orbit interaction is included, this energy gap closes and two Dirac cones form around the Fermi energy, one for the top surface and the other for the bottom surface. As shown in Fig. S4(b), the two Dirac cones

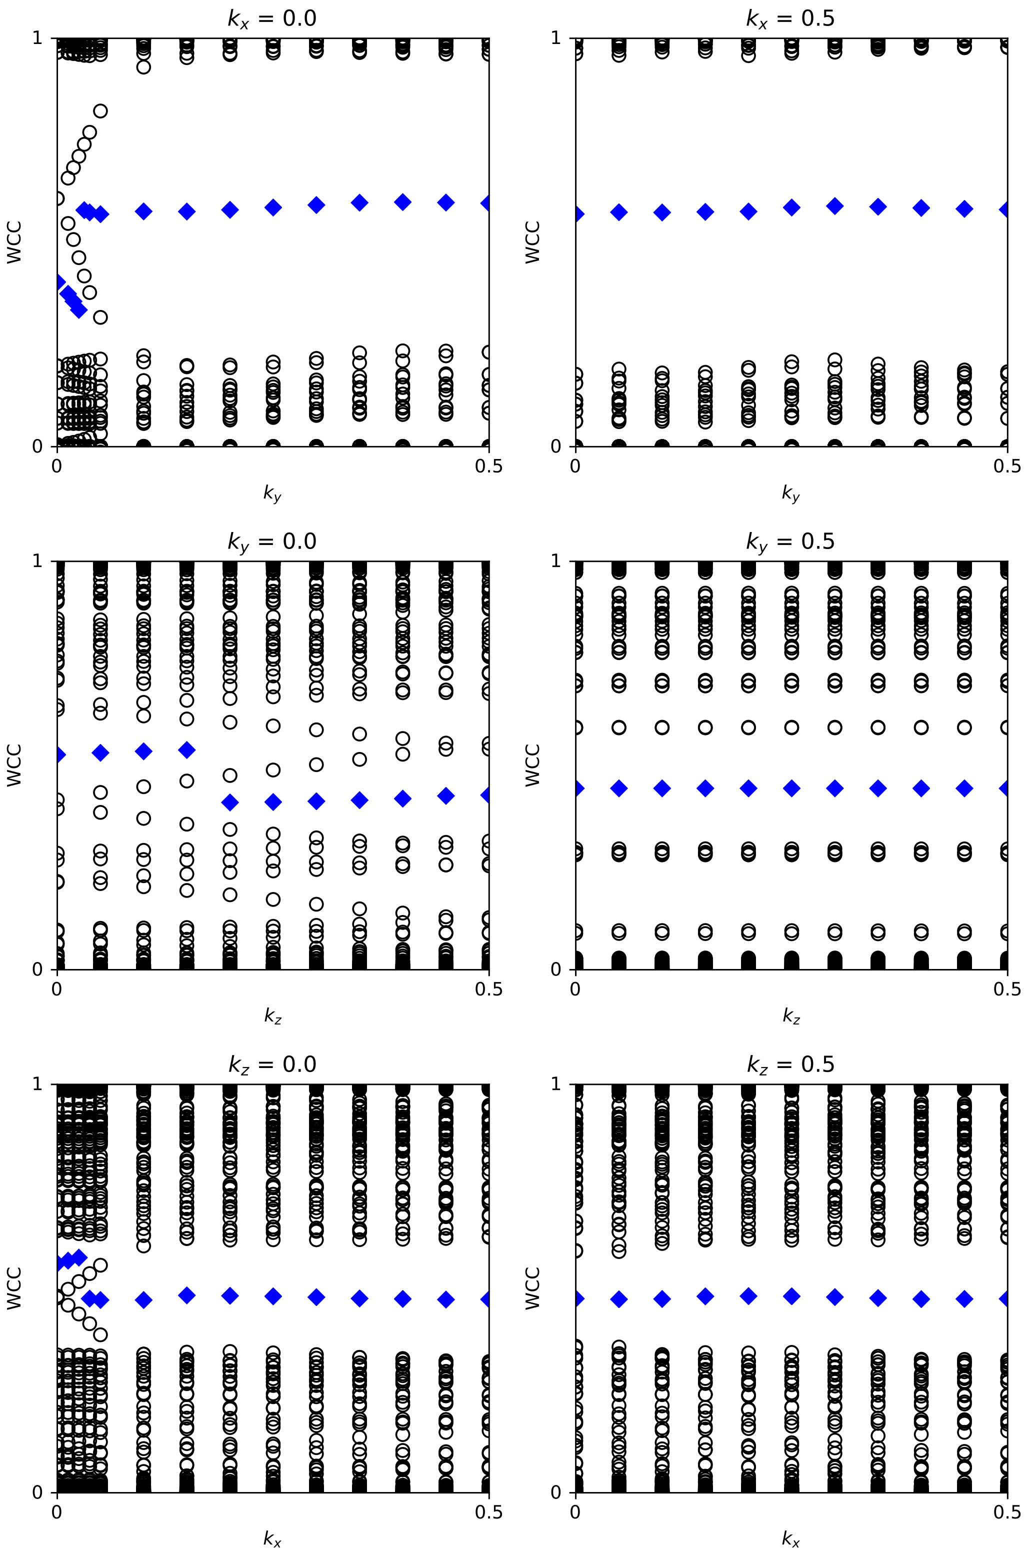


FIG. S3. Hybrid Wannier charge centers (WCC) of the special random BSTS bulk at six reciprocal planes, namely $k_x = 0.0$, $k_x = 0.5$, $k_y = 0.0$, $k_y = 0.5$, $k_z = 0.0$, and $k_z = 0.5$. The WCCs are measured in lattice constants. The wavevectors are in fractional coordinate. Blue diamonds are the middle point of the largest gap between adjacent WCCs.

overlap with each other, since the BSTS slab is inversion symmetric. If we cut a Dirac cone at certain energy, we get a ring of two-component spinors, each of which is localized at the BSTS surface. The corresponding local magnetic moment directs opposite the spin. In Fig. S4(c) [S4(d)], we plot the local magnetic moment $(m_x, m_y)$ along the ring at the energy $E = 0.05\,\mathrm{eV}$. Obviously, $\boldsymbol{m}$ is perpendicular to $\boldsymbol{k}$, and the two surfaces have opposite magnetic moment at the same energy and crystal momentum $(E, \boldsymbol{k})$. Only the in-plane components of the magnetic momentum are considered because the out-of-plane component is much smaller.

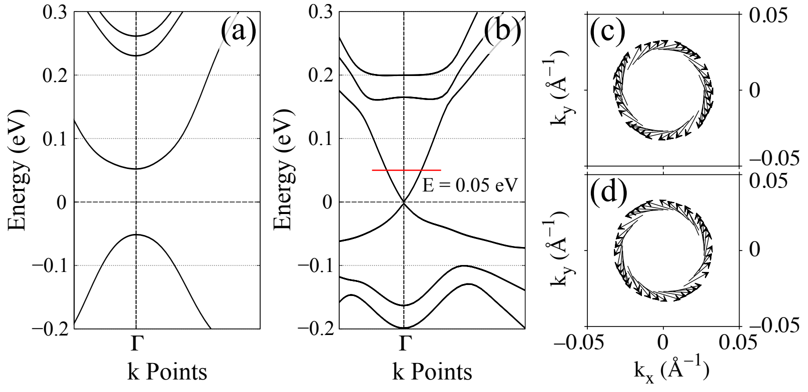


FIG. S4. Band structure of an inversion symmetric BSTS slab (a) without and (b) with spin-orbit interaction. The Fermi energy is set to zero. The red line in panel (b) marks the energy $E = 0.05\,\mathrm{eV}$. Panel (c) [(d)] shows the local magnetic moment at the top surface [the bottom surface] for the surface states with energy $E = 0.05\,\mathrm{eV}$. Each arrow is for one state at a particular $k$ point in the Brillouin zone.

When two BSTS slabs are stacked, the interaction between them can be characterized by the energy gap $E_g$ for the interface states at the $\Gamma$ point. Fig. S5 shows $E_g$ versus the inter-slab distance $d$ of the BSTS interface for the three possible kinds of stacking: the "atop" site, hollow site, and bridge site. $E_g$ is nonzero when the inter-slab distance is small regardless of the stacking, which reflects the absence of topological interface states. As the inter-slab distance increases, the energy gap decreases, until it eventually vanishes at about $d = 6\,\text{Å}$. This is computed for the atop site stacking and the hollow site stacking, and we expect a similar inter-slab critical distance for the bridge site stacking since all the three curves in Fig. S5 have nearly the same trend after $4\,\text{Å}$.

Fig. S6(a) shows the band structure of an asymmetric BSTS slab. A bigger red circle (blue square) represents a state that is more localized at the top surface (bottom surface). As shown in the figure, the Dirac point for the top surface band is below Fermi energy while

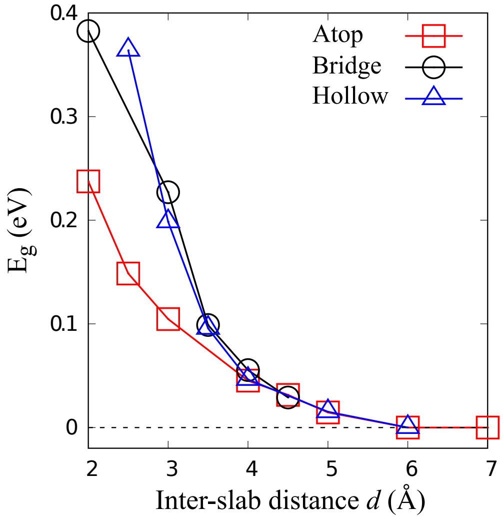


FIG. S5. Band gap at Γ point for the interface states of the BSTS interface versus the inter-slab distance. We consider three different ways of stacking between the two BSTS slabs: the atop site stacking, hollow site stacking and bridge site stacking.

the Dirac point for the bottom surface band is above Fermi energy; in other words, the top surface is doped with electrons and the bottom one is doped with holes. For comparison, we also made an inversion symmetric slab, for which both of the Dirac points are right at the Fermi energy, as shown in Fig. S6(b). Thus the doping effect comes from the asymmetry of the atomic structure. For the asymmetric BSTS slab, the local magnetic momentum is also perpendicular to the wavevector for each surface state, as shown in Fig. S6(c) and (d). For the BSTS/2BN/BSTS structure, Fig. S6(e) and (f) show that spin-momentum locking is still present for the interface states. The spin-momentum locked localized surface/interface states evidence nontrivial topology.

Fig. S7 shows the band structures of BSTS/1BN/BSTS and BSTS/2BN/BSTS with different stackings between BSTS and BN. Two Dirac cones of interface states, one for the top interface and the other for the bottom interface, are present (absent) for BSTS/2BN/BSTS (BSTS/1BN/BSTS), which is true for all examined stackings.

Both VASP and SIESTA are density functional theory based computer packages. The former is generally more accurate than the latter, but some calculations are enabled only in SIESTA. To examine the possible differences, in Fig. S8, we compare the energy bands of a BSTS slab calculated by SIESTA with those calculated by VASP. Qualitative speaking, they match with each other, and the discrepancy for the states above the Fermi level is smaller than that for the states below Fermi energy. It worth mentioning that the Dirac cones are

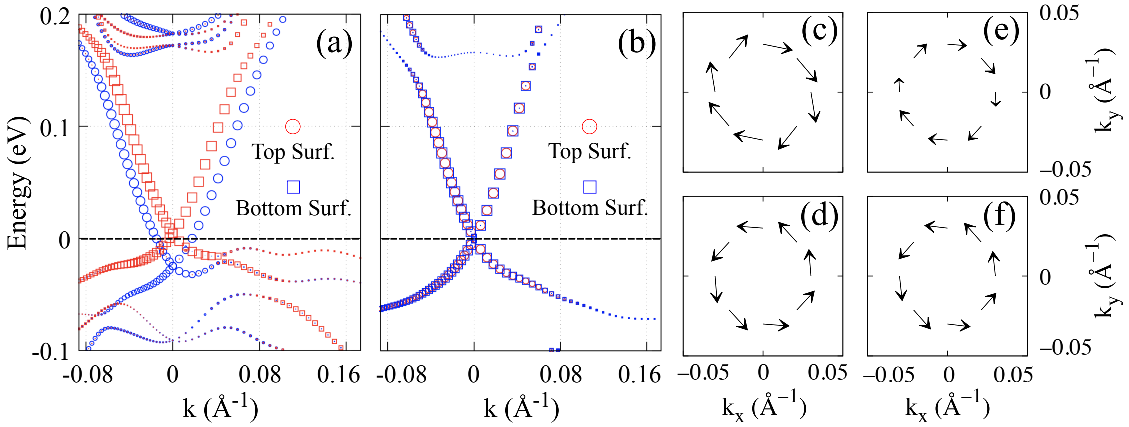


FIG. S6. Band structure of (a) an asymmetric BSTS slab and (b) an inversion symmetric BSTS slab. The size of a red circle (blue square) is proportional to the local density of state projected to the top surface (bottom surface). Panel (c) [(d)] shows the local magnetic moment at the top surface [the bottom surface] for the surface states of the asymmetric slab. The top (bottom) surface states are about 0.05 eV (0.09 eV) below (above) the Fermi level, which is set to zero. Panel (e) [(f)] shows the local magnetic moment at the top interface [the bottom interface] for the interface states of the BSTS/2BN/BSTS structure. The top (bottom) surface states are about 0.02 eV (0.07 eV) below (above) the Fermi level.

captured by both packages. The parameters for the basis set used in SIESTA and the input files for the ATOM code to generate pseudopotentials for Sb, B and N are given towards the end of this document.

As noted in the main text, when the BSTS interface with bilayer BN is subject to a single gate electrode, the doped electrons are mainly at the surface that is closest to the gate electrode, shown in Fig. S9. As a result, the interfacial region is barely doped.

When the BSTS interface with bilayer BN is influenced by dual gates and doped with a net charge $Q$ per unit cell, the charge distribution can be further tuned by the electric field $E$ between the two electrodes. Fig. S10(a) shows the the electron density difference $\rho(Q = -0.05, E = 0.001) - \rho(Q = -0.05, E = 0)$, where the units for $Q$ and $E$ are unit charge and V/Å respectively. Due to the electric field, some electrons move from the top surface to the bottom surface, but the inner part of the heterostructure is barely affected. At a higher electric field $E = 0.02$ V/Å, charge is not only transferred on the surfaces but also appears in the bulk part of the BSTS slab, as shown in Fig. S10(b). Such charge redistribution can be understood by examining the band structure under different electric field. Fig. S10(c)–(f) show the band structure of the BSTS interface with bilayer BN under electric fields of 0, 0.001, 0.005 and 0.02 V/Å respectively. The net charge per cell for

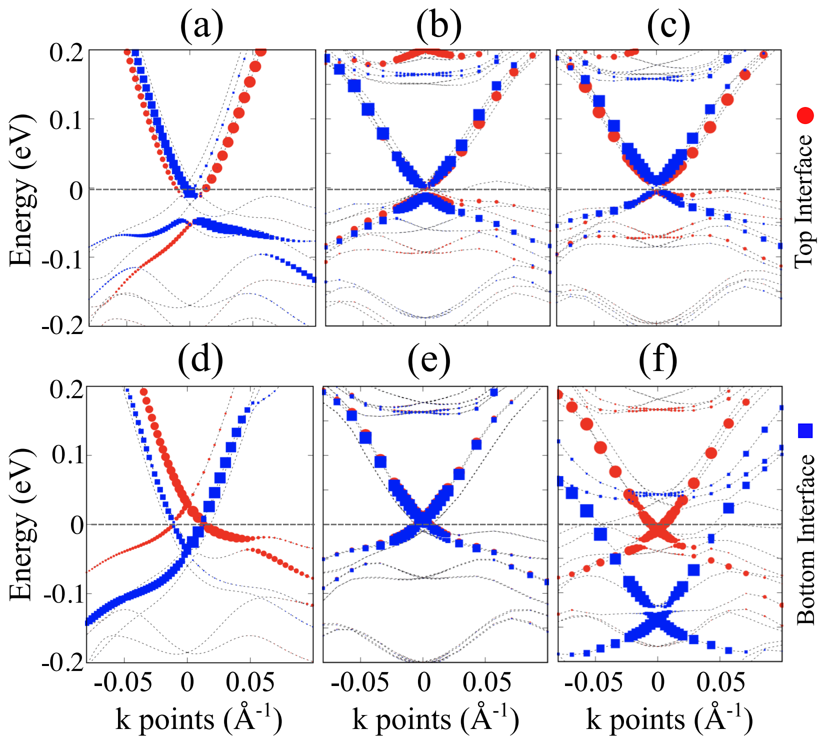


FIG. S7. Band structure of BSTS/1BN/BSTS with (a) hollow site stacking, (b) on-top site stacking, and (c) bridge site stacking between BSTS and BN. Band structure of BSTS/2BN/BSTS with (d) hollow site stacking, (e) on-top site stacking, and (f) bridge site stacking between BSTS and BN. The size of the red circles (the blue squares) is proportional to the projected density of states to the top interface (the bottom interface). Fermi level is set to zero.

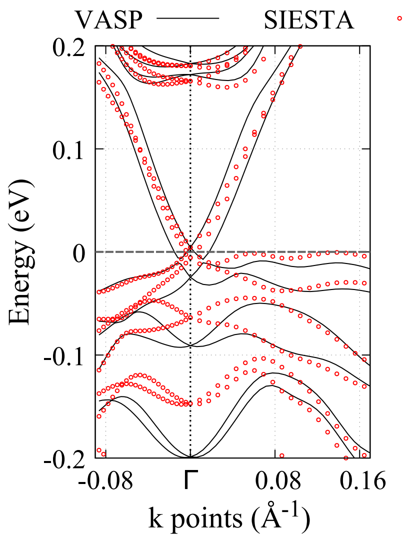


FIG. S8. Band structure of a BSTS slab as calculated by both VASP and SIESTA packages.

these four cases is the same, i.e. $Q = -0.05$ unit charge. The size of an empty/filled red circle is proportional to the local density of states of the top surface/interface. The size

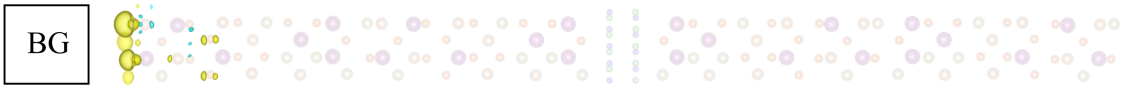


FIG. S9. Distribution of extra electrons for the BSTS interface with bilayer BN when subject to a single gate electrode. The carrier density is $-1.64 \times 10^{13}\,\mathrm{cm}^{-2}$, or 0.05 electrons per unit cell. The isosurface level is $5 \times 10^{-5}\,\mathrm{Bohr}^{-1}$.

of an empty/filled blue square is proportional to the local density of states of the bottom surface/interface. At zero electric field, only the top surface and the bottom surface energy bands are doped with electrons. When a positive electric field is applied, the top (bottom) surface band moves upwards relative to Fermi energy and thus the top (bottom) surface becomes less (more) doped. This is consistent with the charge redistribution shown in Figs. S10(a) and S10(b). The applied electric field also brings the bulk energy bands of the bottom slab closer to Fermi energy. At strong enough electric field, the bulk energy bands of the bottom slab eventually reach the Fermi energy, and the inner part of the BSTS slabs also become doped.

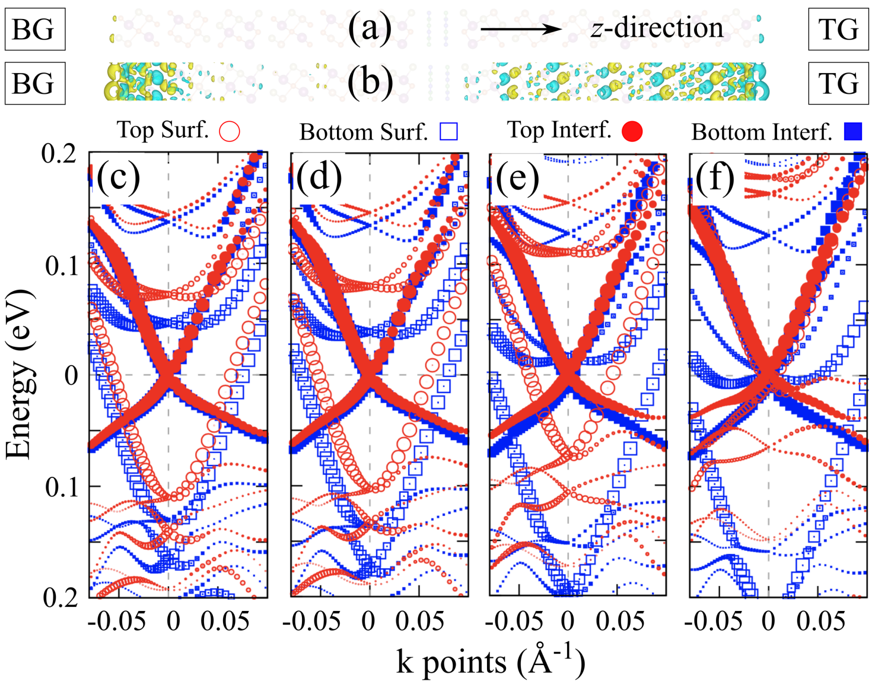


FIG. S10. a) Isosurface of the electron density difference $\rho(Q = -0.05, E = 0.001) - \rho(Q = -0.05, E = 0)$ and b) $\rho(Q = -0.05, E = 0.02) - \rho(Q = -0.05, E = 0)$ with an isosurface value of $5 \times 10^{-6}\,\mathrm{Bohr}^{-3}$ for the BSTS interface with bilayer BN. The direction of the average electric field is indicated by the arrow. c-f) Band structures for the interface under electric fields of 0, 0.001, 0.005 and 0.02 V/Å respectively; the net charge per cell is fixed to $Q = -0.05$ unit charge. The Fermi energy is set to zero and indicated by the horizontal dashed line. The Γ-point is indicated by the vertical dashed line for guiding eyes.

The optimized basis set used in our SIESTA simulations is as follows.

```
%block PAO.Basis
Bi                  2
 n=6   0   1
   5.8210760
   1.000
 n=6   1   1   P  1
   6.5359023
   1.000
Sb                  2
 n=5   0   1
   5.5116770
   1.000
 n=5   1   1   P  1
   6.1141656
   1.000
Se                  2
 n=4   0   1
   5.1773706
   1.000
 n=4   1   1   P  1
   6.0466674
   1.000
Te                  2
 n=5   0   1
   5.8710557
   1.000
 n=5   1   1   P  1
   6.4668471
   1.000
B                   2
 n=2   0   1
   5.5351250
   1.000
 n=2   1   1  P    1
   5.8500000
   1.000
N                   2
 n=2   0   1
   4.7000000
   1.000
 n=2   1   1  P    1
   5.0000000
   1.000
%endblock PAO.Basis
```

The input files for the ATOM code to generate pseudopotentials are as follows.

```
   pe                     -- file generated from Sb ps file
        tm2
   Sb   pbr
     0.000     0.000     0.000     0.000     0.000     0.000
    9    4
    5    0     2.000     0.000    #5s
    5    1     3.000     0.000    #5p
    5    2     0.000     0.000    #5d
    4    3     0.000     0.000    #4f
   2.80000   2.00000   3.25000   2.55000   0.01000  -1.00000 small core charge

#234567890123456789012345678901234567890123456789012345678890      Ruler

   pe                     -- file generated from B ps file
        tm2
    B   pbr
     0.000     0.000     0.000     0.000     0.000     0.000
    1    4
    2    0     2.000     0.000    #2s
    2    1     1.000     0.000    #2p
    3    2     0.000     0.000    #3d
    4    3     0.000     0.000    #4f
   1.74000   1.74000   1.74000   1.74000   0.00000   0.75000 Core corrs

#234567890123456789012345678901234567890123456789012345678890      Ruler

   pe                     -- file generated from N ps file
        tm2
    N   pbr
     0.000     0.000     0.000     0.000     0.000     0.000
    1    4
    2    0     2.000     0.000    #2s
    2    1     3.000     0.000    #2p
    3    2     0.000     0.000    #3d
    4    3     0.000     0.000    #4f
   1.48000   1.48000   1.48000   1.48000   0.01000  -1.00000 small core charge

#234567890123456789012345678901234567890123456789012345678890      Ruler
```

## REFERENCES


[1]A. A. Soluyanov and D. Vanderbilt, Phys. Rev. B **83**, 235401 (2011).
